# Supplementary material for: Using Human Brain Activity to Guide Machine Learning
Source: arXiv:1703.05463 ancillary file (2017-09-19)
Supplement: Supplementary file 1 [file fong-et-al-supplementary.pdf]

# Supplementary Material for “Using human brain activity to guide machine learning”

Ruth C. Fong,<sup>1,3,†</sup> Walter J. Scheirer,<sup>2,3†</sup> David D. Cox<sup>3\*</sup>

<sup>1</sup>Department of Engineering Science, University of Oxford  
Information Engineering Building, Oxford OX1 3PJ, United Kingdom

<sup>2</sup>Department of Computer Science and Engineering, University of Notre Dame  
Fitzpatrick Hall of Engineering, Notre Dame, IN, 46556, USA

<sup>3</sup>Department of Molecular and Cellular Biology, School of Engineering and Applied Sciences  
and Center for Brain Science, Harvard University.  
52 Oxford St., Cambridge, MA, 02138, USA

\*To whom correspondence should be addressed; E-mail: davidcox@fas.harvard.edu.

<sup>†</sup>R.C. Fong and W.J. Scheirer contributed equally to this work.

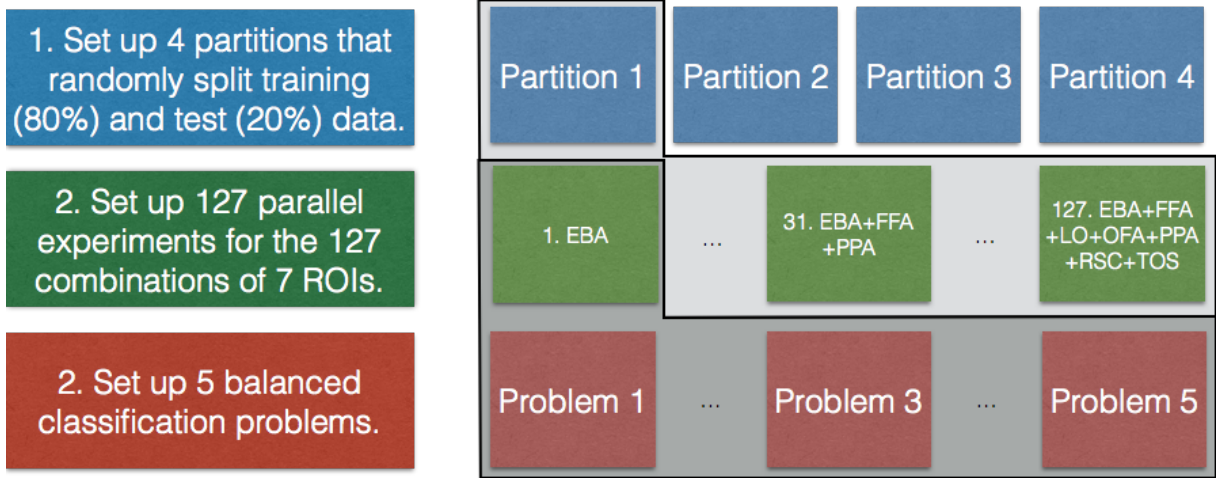

Figure 1: Experimental Design.

## Supplemental Details of Experimental Set-up

Figure 1 outlines the experimental set-up. Using the set of 1386 images that were viewed by subjects in [1], four partitions of training and test splits were randomly generated. There are 127 ways to combine the up to 7 regions of interests (ROIs) associated to high-level visual understanding, i.e. EBA, FFA, LO, OFA, PPA, RSC, TOS, when enumerating all possible combinations of including one to seven ROIs. For each partition, each combination of ROI regions, and each of the four object categories, i.e. humans, animals, buildings, foods, activity weights are generated for all training examples in the clear sample set by using a cross-validated classifier trained on the voxel activity from a given ROI combination (see fMRI Activity Weight Calculation for more details). For each partition, ROI combination, and object category, 5 balanced classification problems were set-up by randomly sampling a partition’s training set to create a balanced training set with the maximally, equal number of positive and negative examples for an object category. This balanced training set is then used to train the baseline hinge loss (HL) classifier and activity weighted loss (AWL) classifier on Histogram of Oriented

Gradients (HOG) features of images in the balanced training set as well as Convolutional Neural Network (CNN) features.

## Supplemental Accuracy Analysis

Additional experiments were conducted to determine how many ROI combinations had activity weights produced results that were statistically significantly better than those from the baseline classifiers with hinge loss. Not only do we observe significant improvements in classification accuracy when activity weights were generated from voxels in all 7 ROIs or from voxels in the EBA, FFA, and PPA regions, we also observe that using activity weights significantly increased classification accuracy when activity weights were generated from most of the 127 ROI combinations of voxels (Figure 2).

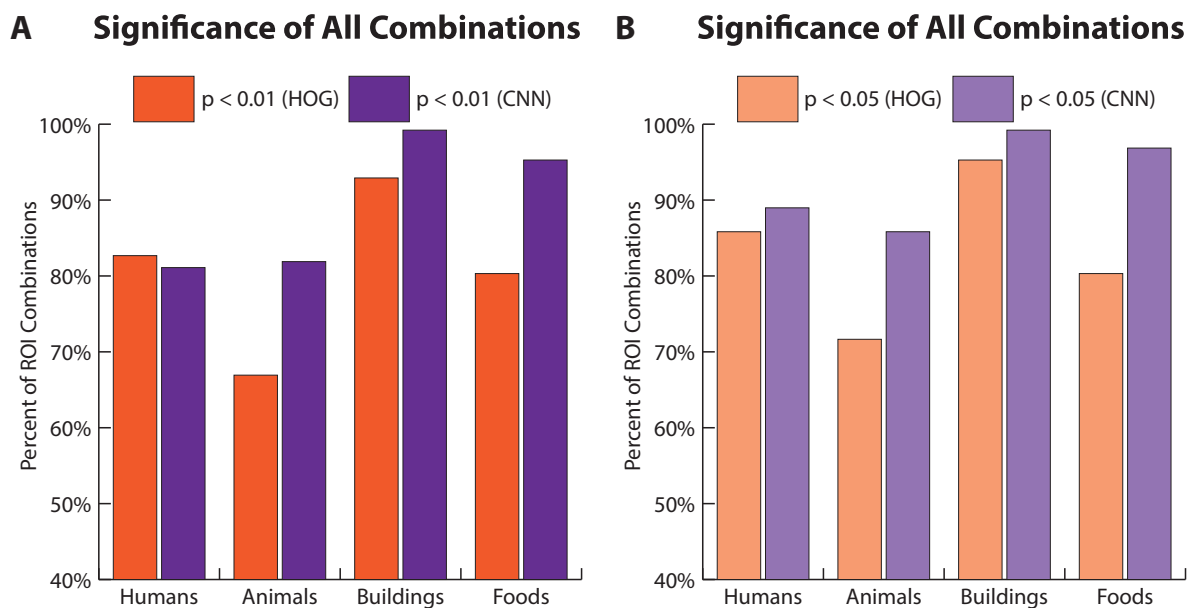

Figure 2: Significance of all combinations of ROIs. The percentage of combinations (out of 127 combinations of ROIs) in which the mean classification accuracy of classifiers that used activity weights was significantly better than that of classifiers that did not use activity weights. One-tailed, paired t-tests were used to test significance.

## Supplemental ROI Analysis

The main text of the paper contains ROI influence plots for biologically-informed classifiers trained with HOG features [2]. Here we present the remaining ROI influence plots for CNN features [3]. Figure 3 shows which ROIs significantly differed from the respective null distributions for each object category. This analysis further confirms the significant impacts of the EBA region in improving the classification of humans and animals and of the PPA region in improving the classification of buildings and foods. Similar to what we observed with the HOG features, the EBA area dramatically exceeds the significance thresholds of the humans and animals null distributions.

## Sequential Minimal Optimization

Sequential Minimal Optimization (SMO) [4] is commonly deployed to solve the quadratic programming problem that follows from the articulation of SVM as an optimization problem. For binary classification, assume a collection of labeled training data points  $(x_1, y_1), \dots, (x_n, y_n)$ , where  $x \in \mathbb{R}^d$  is a feature vector and  $y \in \{-1, 1\}$  is a class label. The dual form of the quadratic programming problem for SVM is:

$$\max_{\alpha} \sum_{i=1}^n \alpha_i - \frac{1}{2} \sum_{i=1}^n \sum_{j=1}^n y_i y_j K(x_i, x_j) \alpha_i \alpha_j,$$

subject to :

$$0 \leq \alpha_i \leq C, \quad \text{for } i = 1, 2, \dots, n,$$

$$\sum_{i=1}^n y_i \alpha_i = 0$$

where  $C$  is a hyperparameter that controls the cost of misclassification,  $K(x_i, x_j)$  is a kernel function, and  $\alpha_i$  are Lagrange multipliers.

SMO treats the above problem as the smallest possible series of sub-problems. For any two

### Analysis of ROIs (CNN)

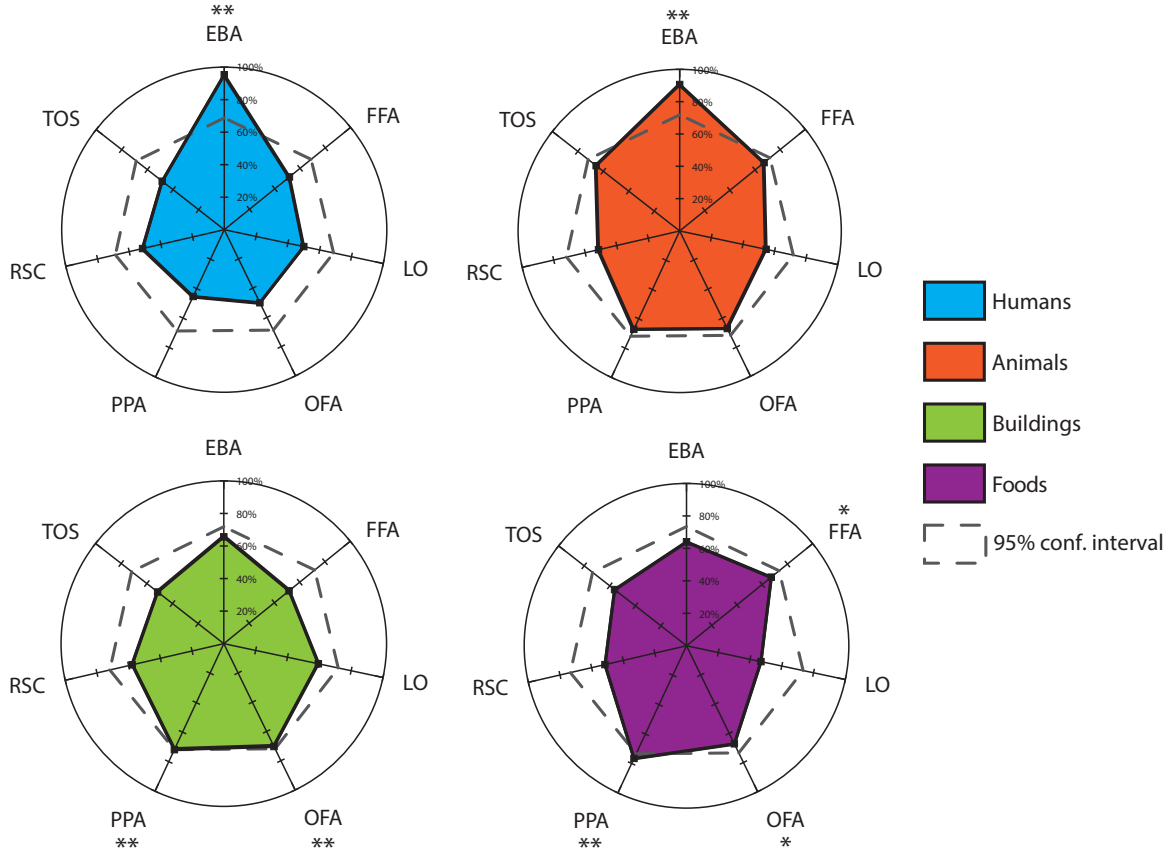

Figure 3: The influence of each ROI for the four object categories (CNN features). In each graph, the fraction of the 64 ROI combinations containing a specific ROI that had a mean classification accuracy greater than that of all 127 sets of experiments is plotted. The threshold for the 95% confidence interval ( $p < 0.0004$ ) is also overlaid, showing which ROIs significantly differed from the respective null distribution for each object category. Bonferroni correction ( $\alpha = 127$ ) is used to account for multiple comparisons.

multipliers  $\alpha_1$  and  $\alpha_2$ , the constraints reduce to:

$$0 \leq \alpha_1, \alpha_2 \leq C$$

$$y_1\alpha_1 + y_2\alpha_2 = k$$

which can be solved analytically to find a minimum of a one-dimensional quadratic function.  $k$  is fixed on each iteration, and is the negative of the sum over the rest of the terms in the equality constraint. The SMO algorithm solves the problem via three steps: (1) find  $\alpha_1$  that violates the Karush-Kuhn-Tucker (KKT) conditions for the optimization problem; (2) pick  $\alpha_2$  and optimize the pair  $(\alpha_1, \alpha_2)$ ; (3) repeat the first two steps until the algorithm converges. To solve the entire optimization problem, this procedure must be applied until all of the Lagrange multipliers satisfy the KKT conditions. By changing the SVM loss function to Eq. 2 in the main paper, the formulation becomes non-convex, with no guarantees on global convergence. However, by design, the optimization finds good local solutions, steered by the activity weights.

## References and Notes

- [1] Stansbury, D., Naselaris, T. & Gallant, J. L. Natural scene statistics account for the representation of scene categories in human visual cortex. *Neuron* **79**, 1025–1034 (2013).
- [2] Vedaldi, A. & Fulkerson, B. VLFeat: An open and portable library of computer vision algorithms. <http://www.vlfeat.org/> (2008).
- [3] Jia, Y. & *et al.* Caffe: Convolutional architecture for fast feature embedding. *CoRR* **abs/1408.5093** (2014). URL <http://arxiv.org/abs/1408.5093>.
- [4] Platt, J. Fast training of support vector machines using sequential minimal optimization. In *Advances in Kernel Methods - Support Vector Learning* (MIT Press, 1998).
